# Supplementary material for: IsoME: Streamlining High-Precision Eliashberg Calculations
Source: arXiv:2503.03559 source file (2025-06-18)
Supplement: Supplementary file 1 [file Suppl.pdf]

# Supplemental Material
# for
# IsoME: Streamlining High-Precision Eliashberg Calculations

Eva Kogler,[1] Dominik Spath,[1] Roman Lucrezi,[1,2] Hitoshi Mori,[3]
Zien Zhu,[4] Zhenglu Li,[4] Elena R. Margine,[3] and Christoph Heil[1,†]

[1]*Institute of Theoretical and Computational Physics,*
*Graz University of Technology, NAWI Graz, 8010, Graz, Austria*
[2]*Department of Materials and Environmental Chemistry,*
*Stockholm University, SE-10691 Stockholm, Sweden*
[3]*Department of Physics, Applied Physics,*
*and Astronomy, Binghamton University-SUNY,*
*Binghamton, New York 13902, USA*
[4]*Mork Family Department of Chemical Engineering and Materials Science,*
*University of Southern California, Los Angeles, California 90089, USA*

(Dated: March 5, 2025)

## I. USAGE OF ISOME

IsoME [1] is a registered Julia package available for installation through various channels. To install IsoME using the Julia package manager, follow these steps:

1. Ensure that you have Julia 1.10 or later installed.

2. Open the Julia REPL and run:

   - `using Pkg`
   - `Pkg.add("IsoME")`

Alternatively, the package can also be obtained from GitHub or Zenodo [1]. Detailed usage instructions and further information are provided in the package documentation.

## II. BENCHMARK AND CONVERGENCE TESTS

For comparison, Tab. I provides the $T_c$ values for materials of our benchmark study, calculated with the default value of $\mu^*_{AD} = 0.12$. Additionally, when available, the results of SCDFT calculation from the literature are included.

TABLE I: Comparison of resulting $T_c$ for different levels of theory within IsoME. $T_c^{AD}$, $T_c^{ML}$, $T_c^{E,\ cdos,\ \mu}$, $T_c^{E,\ vdos,\ \mu}$, $T_c^{exp}$, and $T_c^{SCDFT}$ are the critical superconducting temperatures within McMillan Allen Dynes, the machine learned improvement of it, Migdal-Eliashberg constant DOS and variable DOS using $\mu^*_{AD} = 0.12$, Migdal-Eliashberg variable DOS, the experimental value, and the result obtained from SCDFT, respectively.

| Compound | $T_c^{AD}$ (K) | $T_c^{ML}$ (K) | $T_c^{E,\ cdos,\ \mu}$ (K) | $T_c^{E,\ vdos,\ \mu}$ (K) | $T_c^{exp}$ (K) | $T_c^{SCDFT}$ (K) |
|---|---|---|---|---|---|---|
| Nb | 9 | 9 | 9 | 8 | 9.1-9.5 [2] | 11 [3] |
| Al | 1.0 | 1.0 | 0.5 | 0.5 | 1.2 [2] | 2 [3] |
| Tc | 15 | 14 | 14 | 14 | 8.2-9.3-11.1 [2] | - |
| $\beta$-Sn | 6 | 6 | 5 | 5 | 3.7 [2] | 5 [3] |
| Pb (wSOC) | 7 | 7 | 7 | - | 7.2 [2] | 6 [3] |
| Pb (woSOC) | 8 | 9 | 8 | - | 7.2 [2] | 6 [3] |
| NbC | 14 | 14 | 13 | 13 | 12.8* [4] | - |
| TiN | 13 | 12 | 12 | 12 | 5.6* [2] | - |
| $Nb_2S$ (225 GPa) | 18 | 23 | 19 | - | - | - |
| $H_3S$ (200 GPa) | 228 | 258 | 240 | 221 | 172-184 [5] | 131 [6] |
| $YH_6$ (200 GPa) | 201 | 229 | 224 | 221 | 208-214 [7] | - |
| $LaBeH_8$ (100 GPa) | 120 | 127 | 130 | 131 | 104 [8] | - |
| $LaBH_8$(50 GPa) | 133 | 145 | 138 | 142 | - | - |
| $BaSiH_8$ (30 GPa) | 55 | 59 | 58 | 60 | - | - |

† Corresponding author: christoph.heil@tugraz.at

## III. EQUATIONS

Starting from the most general form of the isotropic Eliashberg equations with static Coulomb interactions [Eq. (13a)-(13d) and Eq. (13e) in the main text], three simpler approximations can be derived, which are also implemented within IsoME. The abbreviations are discussed in Sec. II of the main text.

### A. cDOS W

By assuming a constant DOS around the Fermi energy, the energy shift $\chi(\omega_j)$ vanishes, and the particle number equation is automatically satisfied. The remaining equations then simplify to

$$Z(i\omega_j) = 1 + \frac{\pi}{\beta\omega_j} \sum_{j'=0}^{\infty} \frac{\omega_{j'} Z(i\omega_{j'}) \lambda_{jj'}^{(-)}}{\sqrt{\Theta(0,\omega_{j'})}} \tag{1}$$

$$\phi^{ph}(i\omega_j) = \frac{\pi}{\beta} \sum_{j'=0}^{\infty} \frac{\phi(0,\omega_{j'}) \lambda_{jj'}^{(+)}}{\sqrt{\Theta(0,\omega_{j'})}} \tag{2}$$

$$\begin{aligned}\phi^c(\varepsilon) = -\int d\varepsilon' W(\varepsilon,\varepsilon') N(\varepsilon') \Bigg\{ &\frac{\phi^c(\varepsilon')}{2} \frac{\tanh\left[\frac{\beta}{2}\sqrt{\varepsilon' + \phi^{c2}(\varepsilon')}\right]}{\sqrt{\varepsilon'^2 + \phi^{c2}(\varepsilon')}} \\ + 2k_\mathrm{B}T \sum_{n'=0}^{M} &\left[ \frac{\phi^{ph}(i\omega_{j'}) + \phi^c(\varepsilon')}{\Theta(\varepsilon', i\omega_{j'})} - \frac{\phi^c(\varepsilon')}{\omega_{j'}^2 + \varepsilon'^2 + \phi^{c2}(\varepsilon')} \right] \Bigg\}\end{aligned} \tag{3}$$

$$\phi(\varepsilon, i\omega_j) = \phi^{ph}(i\omega_j) + \phi^c(\varepsilon) \tag{4}$$

$$\Theta(\varepsilon, i\omega_j) = [\omega_j Z(i\omega_j)]^2 + \varepsilon^2 + \phi^2(\varepsilon, i\omega_j) \tag{5}$$

This is similar to the approach followed in Ref. [9].

### B. vDOS $\mu^*$

If the Coulomb repulsion between electrons varies slowly around the Fermi level, it can be approximated with a pseudopotential $\mu^*$ as demonstrated in Ref. [10]. The corresponding equations are given by

$$Z(i\omega_j) = 1 + \frac{k_\mathrm{B}T}{N(\varepsilon_\mathrm{F})\omega_j} \int d\varepsilon N(\varepsilon) \sum_{j'=0}^{\infty} \frac{\omega_{j'} Z(i\omega_{j'})}{\Theta(\varepsilon, i\omega_{j'})} \lambda_{jj'}^{(-)} \tag{6}$$

$$\chi(i\omega_j) = -\frac{k_\mathrm{B}T}{N(\varepsilon_\mathrm{F})} \int d\varepsilon N(\varepsilon) \sum_{j'=0}^{\infty} \frac{\varepsilon - \mu_\mathrm{F} + \chi(i\omega_{j'})}{\Theta(\varepsilon, i\omega_{j'})} \lambda_{jj'}^{(+)} \tag{7}$$

$$\phi(i\omega_j) = \frac{k_\mathrm{B}T}{N(\varepsilon_\mathrm{F})} \int d\varepsilon N(\varepsilon) \sum_{j'=0}^{\infty} \frac{\phi(i\omega_{j'})}{\Theta(\varepsilon, i\omega_{j'})} [\lambda_{jj'}^{(+)} - 2\mu^*] \tag{8}$$

$$N_e = \int d\varepsilon N(\varepsilon)\left[1 - 2k_\mathrm{B}T\sum_j \frac{\varepsilon - \mu_\mathrm{F} + \chi(i\omega_j)}{\Theta(\varepsilon, i\omega_j)}\right]$$
$$\approx 2n_\mathrm{F}(\varepsilon - \mu_\mathrm{F}) - 4k_\mathrm{B}T\sum_{j=0}^{\omega_j\leq\omega_\mathrm{c}}\left[\frac{\varepsilon - \mu_\mathrm{F} + \chi(i\omega_j)}{\Theta(\varepsilon, i\omega_j)} - \frac{\varepsilon - \mu_\mathrm{F}}{\omega_j^2 + (\varepsilon - \mu_\mathrm{F})^2}\right] \tag{9}$$

$$\Theta(\varepsilon, i\omega_j) = [\omega_j Z(i\omega_j)]^2 + [\varepsilon - \mu_\mathrm{F} + \chi(i\omega_j)]^2 + [\phi(i\omega_j)]^2 \tag{10}$$

where

$$\lambda_{jj'}^{(\pm)} = \lambda(i\omega_j - i\omega_{j'}) \pm \lambda(i\omega_j + i\omega_{j'}) \tag{11}$$

are differences of the electron-phonon coupling parameter [11]. These equations are derived in Ref. [12].

### C. cDOS $\mu^*$

Combining both of the previously mentioned approximations leads to

$$Z(i\omega_j) = 1 + \frac{\pi k_\mathrm{B}T}{\omega_j}\sum_{j'=-\infty}^{\infty}\frac{\omega_{j'}Z(\omega_{j'})}{\sqrt{\omega_{j'}^2 Z^2(\omega_{j'}) + \phi^2(i\omega_{j'})}}\lambda(i\omega_j - i\omega_{j'})$$
$$= 1 + \frac{\pi k_\mathrm{B}T}{\omega_j}\sum_{j'=0}^{\infty}\frac{\omega_{j'}Z(\omega_{j'})}{\sqrt{\omega_{j'}^2 Z^2(\omega_{j'}) + \phi^2(i\omega_{j'})}}\lambda_{jj'}^{(-)} \tag{12}$$

$$\phi(i\omega_j) = \pi k_\mathrm{B}T\sum_{j'=-\infty}^{\infty}\frac{\phi(i\omega_{j'})}{\sqrt{\omega_{j'}^2 Z^2(\omega_{j'}) + \phi^2(i\omega_{j'})}}[\lambda(i\omega_j - i\omega_{j'}) - \mu^*]$$
$$= \pi k_\mathrm{B}T\sum_{j'=0}^{\infty}\frac{\phi(i\omega_{j'})}{\sqrt{\omega_{j'}^2 Z^2(\omega_{j'}) + \phi^2(i\omega_{j'})}}[\lambda_{jj'}^{(+)} - 2\mu^*]\ . \tag{13}$$

## IV. SEMI-EMPIRICAL EQUATIONS FOR $T_\mathrm{c}$

The McMillan equation [13] provides a direct but approximate method to calculate $T_\mathrm{c}$ based on empirically derived parameters. With small modifications done by Dynes [14], $T_\mathrm{c}$ is given by:

$$T_\mathrm{c}^\mathrm{McM} = \frac{\omega_\mathrm{log}}{1.2}\exp\left(-\frac{1.04(1+\lambda)}{\lambda - \mu^*(1+0.62\lambda)}\right), \tag{14}$$

where the logarithmic average of the electron-phonon spectral function $\omega_\mathrm{log}$ and the electron-phonon coupling strength $\lambda$ are defined as

$$\omega_\mathrm{log} = \exp\left(\frac{2}{\lambda}\int_0^\infty \frac{\alpha^2F(\omega)}{\omega}\ln(\omega)\,d\omega\right), \tag{15}$$

$$\lambda = \int_0^\infty d\omega\frac{\alpha^2F(\Omega)}{\omega}\ . \tag{16}$$

The expression for $\alpha^2F(\Omega)$ is given in the main text Eq. (11), and $\mu^*$ is the semi-empirical Coulomb pseudopotential.

Allen and Dynes [15] added prefactors to optimize Eq. (14):

$$T_c^{AD} = f_1 f_2 T_c^{McM}, \tag{17}$$

with $f_1$ and $f_2$ defined by

$$f_1 = \left[1 + \frac{\lambda}{2.46}(1+3.8\mu^*)^{3/2}\right]^{1/3}, \tag{18}$$

$$f_2 = 1 + \frac{\left(\frac{\omega_2}{\omega_{\log}} - 1\right)\lambda^2}{\lambda^2 + \left[1.82(1+6.3\mu^*)\frac{\omega_2}{\omega_{\log}}\right]^2}, \tag{19}$$

and $\omega_2$ by:

$$\omega_2 = \frac{2}{\lambda}\int_0^\infty \alpha^2F(\omega)\,\omega\,d\omega. \tag{20}$$

Eq. (17) was further improved using machine learning to get the following expression for a more accurate description, especially for high-$T_c$ hydride superconductors [16]:

$$T_c^{ML} = f_\omega f_\mu T_c^{McM}, \tag{21}$$

with the prefactors

$$f_\omega = 1.92\left[\frac{\lambda + \frac{\omega_{\log}}{\omega_2} - \sqrt[3]{\mu^*}}{\sqrt{\lambda}\cdot\exp\left(\frac{\omega_{\log}}{\omega_2}\right)}\right] - 0.08, \tag{22}$$

and

$$f_\mu = \frac{6.86\exp\left(\frac{-\lambda}{\mu^*}\right)}{\frac{1}{\lambda} - \mu^* - \frac{\omega_{\log}}{\omega_2}} + 1. \tag{23}$$

## V. DERIVATION OF THE ELECTRON NUMBER EQUATION

### A. Non-interacting electrons

In the case of non-interacting (NI) electrons, the electron number can be calculated via

$$\begin{aligned} N_e^{NI} &= 2\int d\varepsilon\, N(\varepsilon) n_F(\varepsilon - \varepsilon_F) \\ &= \int d\varepsilon\, N(\varepsilon)\left[1 - 2k_BT\sum_{j=-\infty}^{\infty}\frac{\varepsilon-\varepsilon_F}{\omega_j^2 + (\varepsilon-\varepsilon_F)^2}\right], \end{aligned} \tag{24}$$

where $N(\varepsilon)$ is the density of states per spin, $n_F$ is the Fermi distribution function, and $\omega_j$ are the fermionic Matsubara frequencies. Even though both formulations are equivalent,

evaluating Eq. (24) through the Fermi function is numerically much more stable. At moderate temperatures, convergence is achieved almost immediately due to the sharp drop in the Fermi function. The summation however has to be truncated at some point, resulting in an additional error $S^{\mathrm{NI}}_{\mathrm{tail}}(\varepsilon, \varepsilon_{\mathrm{F}})$

$$\begin{aligned} 2n_{\mathrm{F}}(\varepsilon-\varepsilon_{\mathrm{F}}) &= 1 - 2k_{\mathrm{B}}T \sum_{j=-\infty}^{\infty} \frac{\varepsilon-\varepsilon_{\mathrm{F}}}{\omega_j^2 + (\varepsilon-\varepsilon_{\mathrm{F}})^2} \\ &= 1 - 2\cdot 2k_{\mathrm{B}}T \sum_{j=0}^{\infty} \frac{\varepsilon-\varepsilon_{\mathrm{F}}}{\omega_j^2 + (\varepsilon-\varepsilon_{\mathrm{F}})^2} \\ &= 1 - 4k_{\mathrm{B}}T \sum_{j=0}^{\omega_j\leq\omega_{\mathrm{c}}} \frac{\varepsilon-\varepsilon_{\mathrm{F}}}{\omega_j^2 + (\varepsilon-\varepsilon_{\mathrm{F}})^2} \underbrace{-4k_{\mathrm{B}}T \sum_{\omega_j>\omega_{\mathrm{c}}}^{\infty} \frac{\varepsilon-\varepsilon_{\mathrm{F}}}{\omega_j^2 + (\varepsilon-\varepsilon_{\mathrm{F}})^2}}_{:=S^{\mathrm{NI}}_{\mathrm{tail}}(\varepsilon,\varepsilon_{\mathrm{F}})} . \end{aligned} \tag{25}$$

Rearranging for the tail gives an estimate of the error

$$S^{\mathrm{NI}}_{\mathrm{tail}}(\varepsilon, \varepsilon_{\mathrm{F}}) = 2n_{\mathrm{F}}(\varepsilon-\varepsilon_{\mathrm{F}}) - 1 + 4k_{\mathrm{B}}T \sum_{j=0}^{\omega_j\leq\omega_{\mathrm{c}}} \frac{\varepsilon-\varepsilon_{\mathrm{F}}}{\omega_j^2 + (\varepsilon-\varepsilon_{\mathrm{F}})^2} . \tag{26}$$

### B. Superconducting phase

In the superconducting phase (SC), the number of electrons can be obtained through a generalization of Eq. (24):

$$N_{\mathrm{e}}^{\mathrm{SC}} = \int \mathrm{d}\varepsilon\, N(\varepsilon) \left[ 1 - 2k_{\mathrm{B}}T \sum_{j=-\infty}^{\infty} \frac{\varepsilon - \mu_{\mathrm{F}} + \chi(i\omega_j)}{\theta(\varepsilon, i\omega_j)} \right] , \tag{27}$$

where the denominator is defined as

$$\Theta(\varepsilon, i\omega_j) = [\omega_j Z(i\omega_j)]^2 + [\varepsilon - \mu_{\mathrm{F}} + \chi(i\omega_j)]^2 + [\phi(\varepsilon, i\omega_j)]^2 . \tag{28}$$

Splitting the sum again at $\omega_{\mathrm{c}}$ and exploiting the fact that all self-energy components are even functions of $\omega_j$ gives an expression for the summation error:

$$\begin{aligned} 1 - 2k_{\mathrm{B}}T \sum_{j=-\infty}^{\infty} \frac{\varepsilon - \mu_{\mathrm{F}} + \chi(i\omega_j)}{\theta(\varepsilon, i\omega_j)} &= 1 - 2\cdot 2k_{\mathrm{B}}T \sum_{j=0}^{\infty} \frac{\varepsilon - \mu_{\mathrm{F}} + \chi(i\omega_j)}{\theta(\varepsilon, i\omega_j)} \\ &= 1 - 4k_{\mathrm{B}}T \sum_{j=0}^{\omega_j\leq\omega_{\mathrm{c}}} \frac{\varepsilon - \mu_{\mathrm{F}} + \chi(i\omega_j)}{\theta(\varepsilon, i\omega_j)} \underbrace{-4k_{\mathrm{B}}T \sum_{\omega_j>\omega_{\mathrm{c}}}^{\infty} \frac{\varepsilon - \mu_{\mathrm{F}} + \chi(i\omega_j)}{\theta(\varepsilon, i\omega_j)}}_{:=S^{\mathrm{SC}}_{\mathrm{tail}}(\varepsilon,\mu_{\mathrm{F}})} . \end{aligned} \tag{29}$$

Above the Matsubara frequency cutoff $\omega_{\mathrm{c}}$, it is safe to assume that $Z(i\omega_j) = 1$, $\chi(i\omega_j) = 0$, $\phi^{ph}(i\omega_j) = 0$ and that the Coulomb contribution to the order parameter $\phi^c(\varepsilon) = 0$ can be

neglected. This allows us to approximate the superconducting tail by the non-interacting tail in Eq. (26) as a function of the Fermi level $S^{\mathrm{NI}}_{\mathrm{tail}}(\varepsilon, \varepsilon_{\mathrm{F}}) \mapsto S^{\mathrm{NI}}_{\mathrm{tail}}(\varepsilon, \mu_{\mathrm{F}}) \approx S^{\mathrm{SC}}_{\mathrm{tail}}(\varepsilon, \mu_{\mathrm{F}})$ leading to:

$$\begin{aligned} 1 - 2T \sum_{j=-\infty}^{\infty} \frac{\varepsilon - \mu_{\mathrm{F}} + \chi(i\omega_j)}{\theta(\varepsilon, i\omega_j)} &\approx 1 - 4k_{\mathrm{B}}T \sum_{j=0}^{\omega_j \leq \omega_c} \frac{\varepsilon - \mu_{\mathrm{F}} + \chi(i\omega_j)}{\theta(\varepsilon, i\omega_j)} + S^{\mathrm{NI}}_{\mathrm{tail}}(\varepsilon, \mu_{\mathrm{F}}) \\ &= 2n_{\mathrm{F}}(\varepsilon - \mu_{\mathrm{F}}) - 4k_{\mathrm{B}}T \sum_{j=0}^{\omega_j \leq \omega_c} \left[ \frac{\varepsilon - \mu_{\mathrm{F}} + \chi(i\omega_j)}{\theta(\varepsilon, i\omega_j)} - \frac{\varepsilon - \mu_{\mathrm{F}}}{\omega_j^2 + (\varepsilon - \mu_{\mathrm{F}})^2} \right] . \end{aligned} \tag{30}$$

Inserting this into Eq. (27) yields

$$N_{\mathrm{e}}^{\mathrm{SC}} = \int \mathrm{d}\varepsilon \, N(\varepsilon) \left\{ 2n_{\mathrm{F}}(\varepsilon - \mu_{\mathrm{F}}) - 4k_{\mathrm{B}}T \sum_{j=0}^{\omega_j \leq \omega_c} \left[ \frac{\varepsilon - \mu_{\mathrm{F}} + \chi(i\omega_j)}{\theta(\varepsilon, i\omega_j)} - \frac{\varepsilon - \mu_{\mathrm{F}}}{\omega_j^2 + (\varepsilon - \mu_{\mathrm{F}})^2} \right] \right\} , \tag{31}$$

which enables a more robust evaluation of the chemical potential. Based on numerical tests, this approach requires much lower Matsubara frequency cutoffs.

### C. $\mu$-update

When performing calculations within the variable DOS approximation, the conservation of electron number must be enforced by updating the chemical potential such that

$$f(\mu_{\mathrm{F}}) = N_{\mathrm{e}}^{\mathrm{NI}} - N_{\mathrm{e}}^{\mathrm{SC}}(\mu_{\mathrm{F}}) \stackrel{!}{=} 0 \tag{32}$$

is satisfied. $N_{\mathrm{e}}^{\mathrm{SC}}(\mu_{\mathrm{F}})$ is a monotonic function of the chemical potential, guaranteeing a unique solution. However, monotonicity is easily violated when introducing a finite Matsubara frequency cutoff in the definition of $N_{\mathrm{e}}^{\mathrm{SC}}$. Using Eq. (31) instead of Eq. (27), ensures both faster convergence of the chemical potential and uniqueness of the root already at much lower cutoffs.

## SUPPLEMENTARY REFERENCES


[1] IsoME is available as a registered Julia package (juliahub.com/ui/Packages/General/IsoME), on GitHub (github.com/cheil/IsoME.jl), and Zenodo (DOI:10.5281/zenodo.14967551).
[2] B. T. Matthias, T. H. Geballe, and V. B. Compton, Rev. Mod. Phys. **35**, 1 (1963).
[3] C. Pellegrini and A. Sanna, Nature Reviews Physics **6** (2024).
[4] A. L. Giorgi, E. G. Szklarz, E. K. Storms, A. L. Bowman, and B. T. Matthias, Phys. Rev. **125**, 837 (1962).
[5] A. P. Drozdov, M. I. Eremets, I. A. Troyan, V. Ksenofontov, and S. I. Shylin, Nature **525**, 73 (2015), publisher: Nature Publishing Group.
[6] J. A. Flores-Livas, A. Sanna, and E. Gross, The European Physical Journal B **89**, 1 (2016).
[7] P. Kong, V. S. Minkov, M. A. Kuzovnikov, A. P. Drozdov, S. P. Besedin, S. Mozaffari, L. Balicas, F. F. Balakirev, V. B. Prakapenka, S. Chariton, *et al.*, Nature communications **12**, 5075 (2021).

[8] Y. Song, J. Bi, Y. Nakamoto, K. Shimizu, H. Liu, B. Zou, G. Liu, H. Wang, and Y. Ma, Phys. Rev. Lett. **130**, 266001 (2023).

[9] C. Pellegrini, R. Heid, and A. Sanna, Journal of Physics: Materials **5**, 024007 (2022), publisher: IOP Publishing.

[10] D. J. Scalapino, J. R. Schrieffer, and J. W. Wilkins, Phys. Rev. **148**, 263 (1966).

[11] W. E. Pickett, Physical Review B **26**, 1186 (1982), publisher: American Physical Society.

[12] H. Lee, S. Poncé, K. Bushick, S. Hajinazar, J. Lafuente-Bartolome, J. Leveillee, C. Lian, J.-M. Lihm, F. Macheda, H. Mori, H. Paudyal, W. H. Sio, S. Tiwari, M. Zacharias, X. Zhang, N. Bonini, E. Kioupakis, E. R. Margine, and F. Giustino, npj Computational Materials **9**, 1 (2023), publisher: Nature Publishing Group.

[13] W. L. McMillan, Phys. Rev. **167**, 331 (1968).

[14] R. C. Dynes, Solid State Communications **10**, 615 (1972).

[15] P. B. Allen and R. C. Dynes, Phys. Rev. B **12**, 905 (1975).

[16] S. R. Xie, Y. Quan, A. C. Hire, B. Deng, J. M. DeStefano, I. Salinas, U. S. Shah, L. Fanfarillo, J. Lim, J. Kim, G. R. Stewart, J. J. Hamlin, P. J. Hirschfeld, and R. G. Hennig, npj Computational Materials **8**, 14 (2022).
